# Supplementary material for: Interpretable Graph Neural Networks for Connectome-Based Brain Disorder Analysis
Source: arXiv:2207.00813 source file (2022-07-23)
Supplement: Supplementary file 1 [file appendix.tex]

\section{Detailed Configuration}
\label{sec:supp-setting}
Table \ref{tab:config} shows the range of hyper-parameters that are examined and the final specification of all hyper-parameters that are utilized to generate the reported results. Both the backbone prediction model and the explanation generator are trained for 100 epochs, and the explanation enhanced prediction model is further tuned for another 50 epochs. All the remaining hyper-parameters are selected automatically with the open-source AutoML toolkit NNI\footref{nni}. The final specification of node feature (edge profile) implies using the corresponding row in the edge weight matrix as the node's initial embedding.

\begin{table}[h]
\centering
\caption{The range of hyper-parameters examined in the experiments and the final specification for the reported performance.}
\label{tab:config}
\resizebox{\linewidth}{!}{
\begin{tabular}{@{}cccc@{}}
\toprule
Hyper-parameter & Range Examined & Final Specification  \\
\midrule
\#GNN Layers & [1,2,3,4] & 2 \\
\#MLP Layers & [1,2,3,4] & 1 \\
Hidden Dimension & [8,12,16,32] & 16 \\
Batch Size & [8,16,32] &  16 \\
Learning Rate  & [$1\mathrm{e}{-1},1\mathrm{e}{-2},1\mathrm{e}{-3},1\mathrm{e}{-4}$] & $1\mathrm{e}{-3}$\\
Weight Decay & [$1\mathrm{e}{-3},1\mathrm{e}{-4},1\mathrm{e}{-5}$] & $1\mathrm{e}{-5}$ \\
Node Feature & [identity, eigen, degree profile, node2vec, edge profile] & edge profile \\
\bottomrule
\end{tabular}
}
\end{table}

\section{Hyper-parameter Sensitivity}
We alter two hyper-parameters in our proposed IBGNN and IBGNN\texttt{+}, namely the number of GNN layers $L$ and the hidden dimension $d$ in the feature encoder, both of which are critical to the model's performance. As seen in the Fig. \ref{fig:sensitivity_vis}, increasing the number of GNN layers or hidden dimension does not always improve the performance, proving the stability of IBGNN and IBGNN\texttt{+}. As the number of GNN layers increases, the diminishing trend may arise from the well-known over-smoothing issue of GNNs. Furthermore, it is impressive that our explanation enhanced model IBGNN\texttt{+} consistently outperforms the backbone when the hyper-parameters are varied.

\label{sec:supp-sensitivity}
\begin{figure}[H]
\centering
    \begin{minipage}{.5\textwidth}
      \centering
      \includegraphics[width=0.85\linewidth]{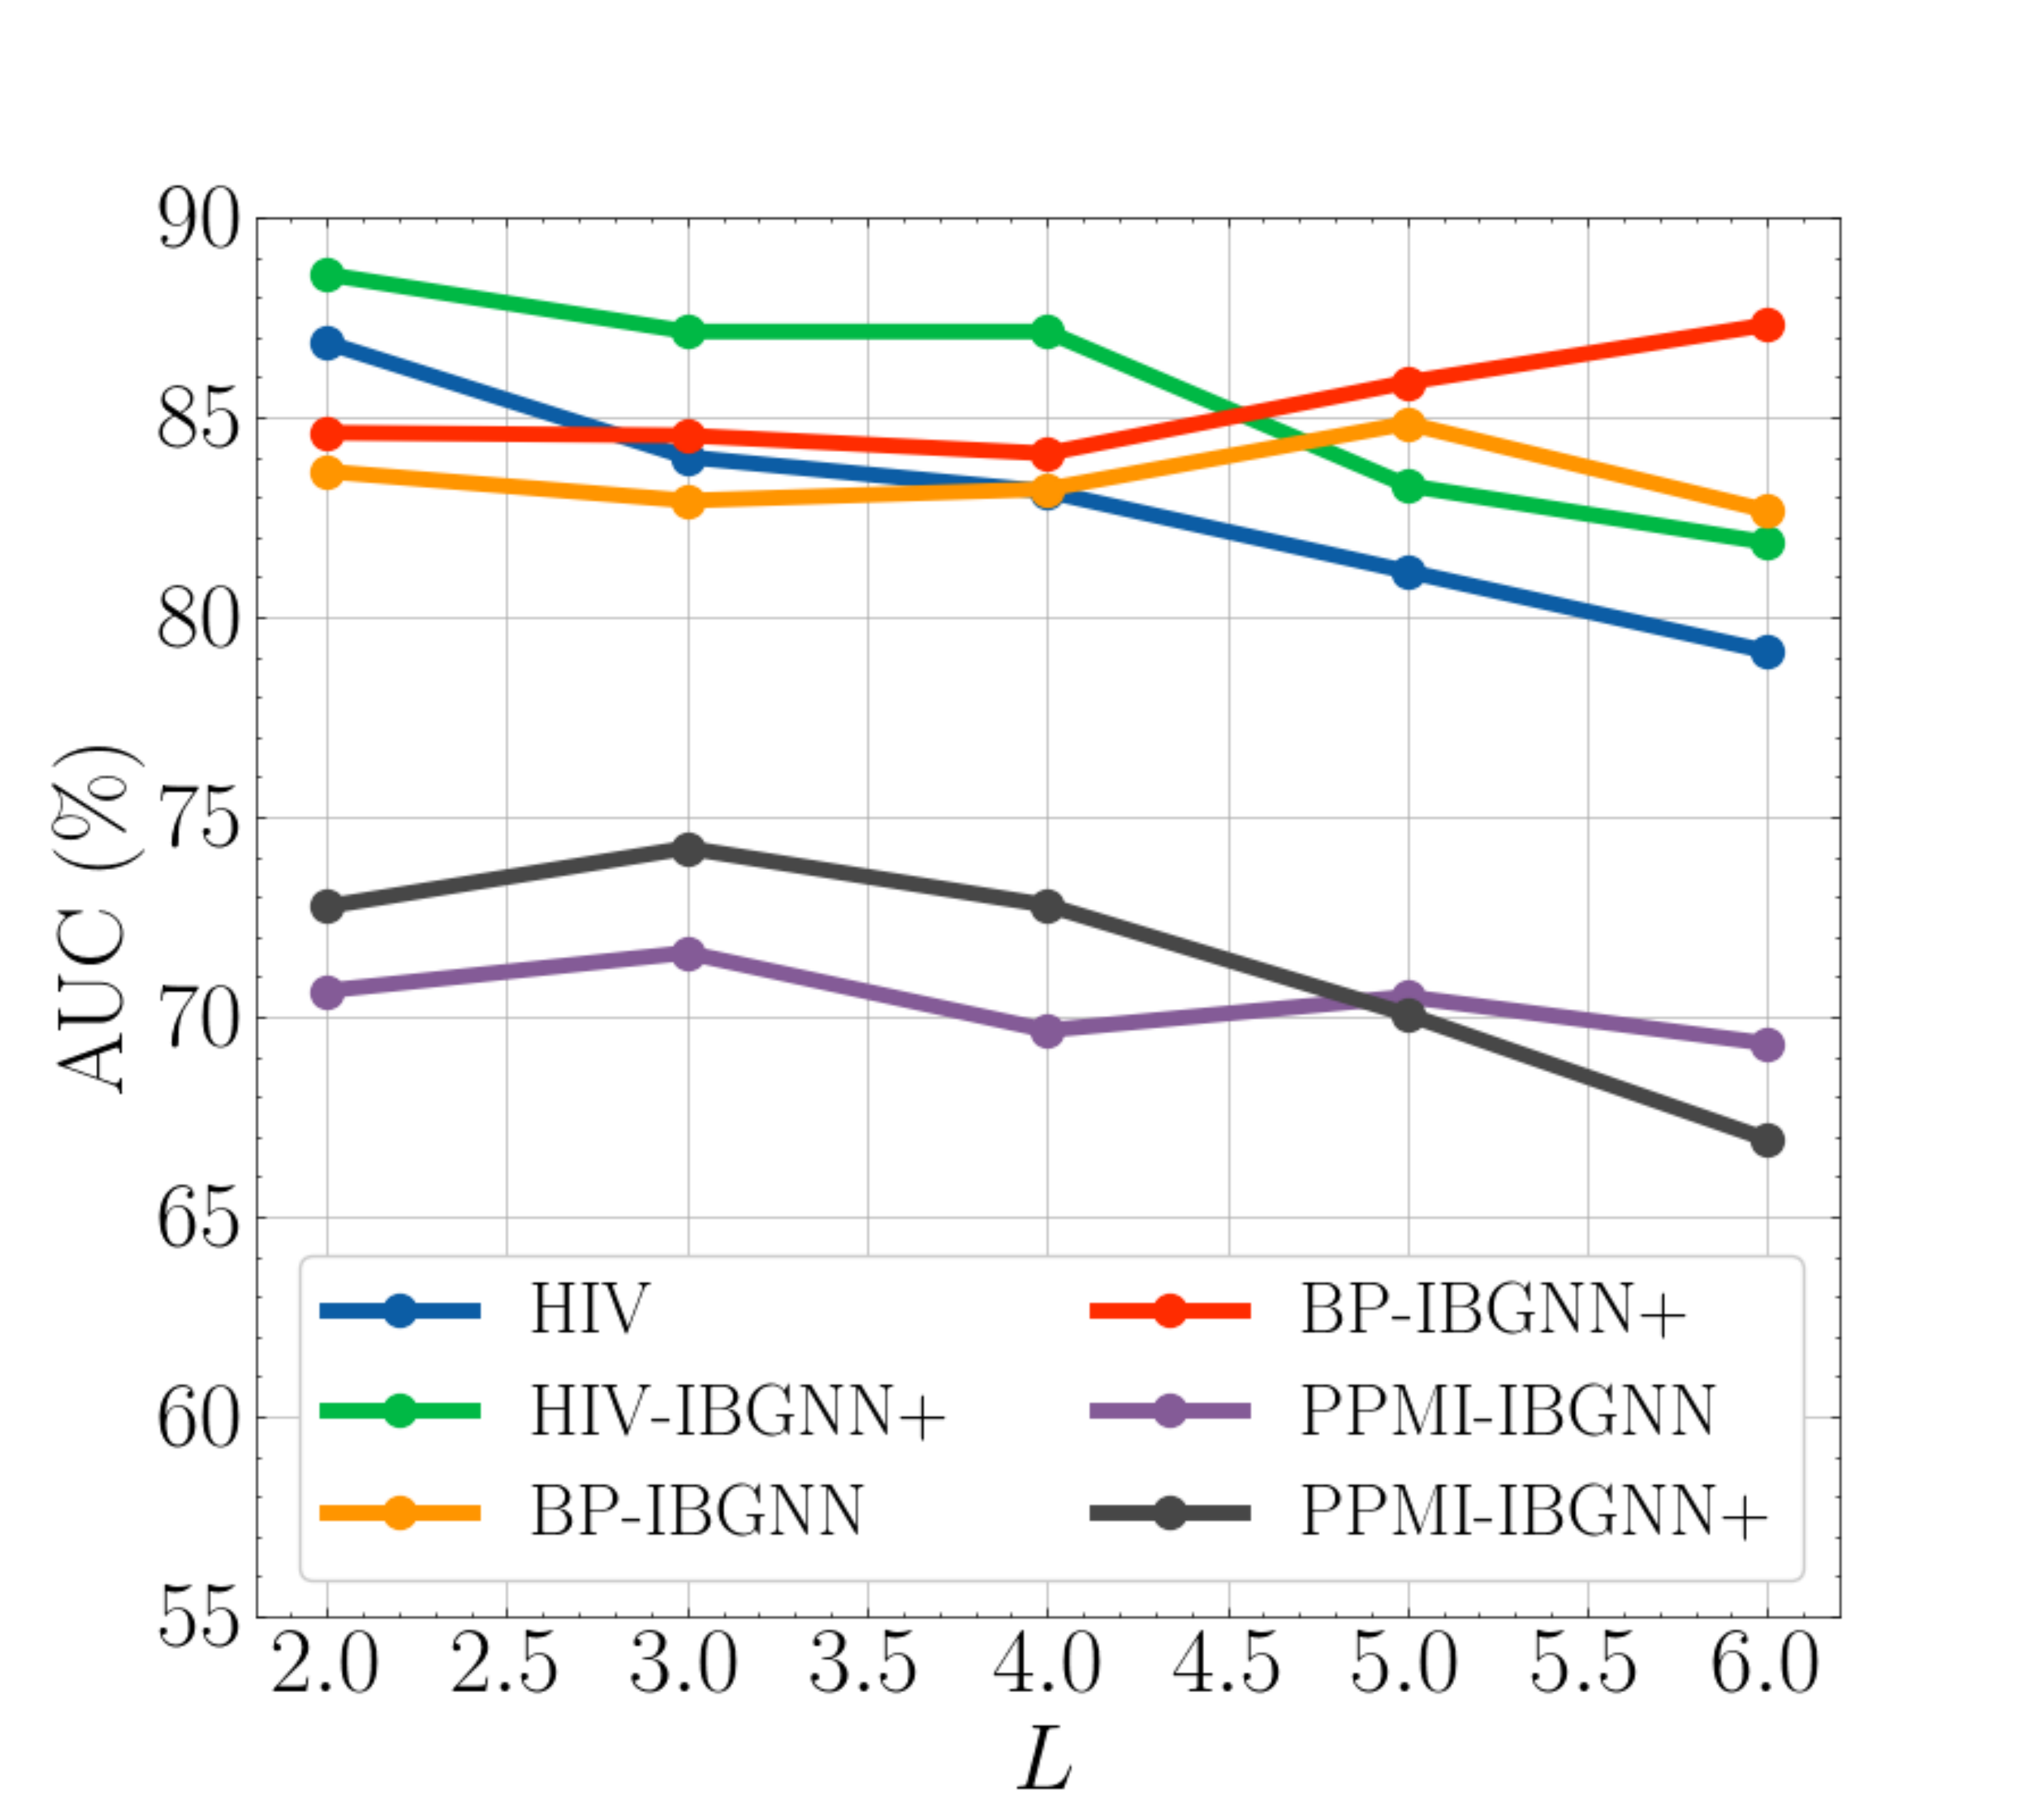}
      
      (a) Number of GNN layers
      \label{fig:hiv_hc_nii}
    \end{minipage}%
    \begin{minipage}{.5\textwidth}
      \centering
      \includegraphics[width=0.85\linewidth]{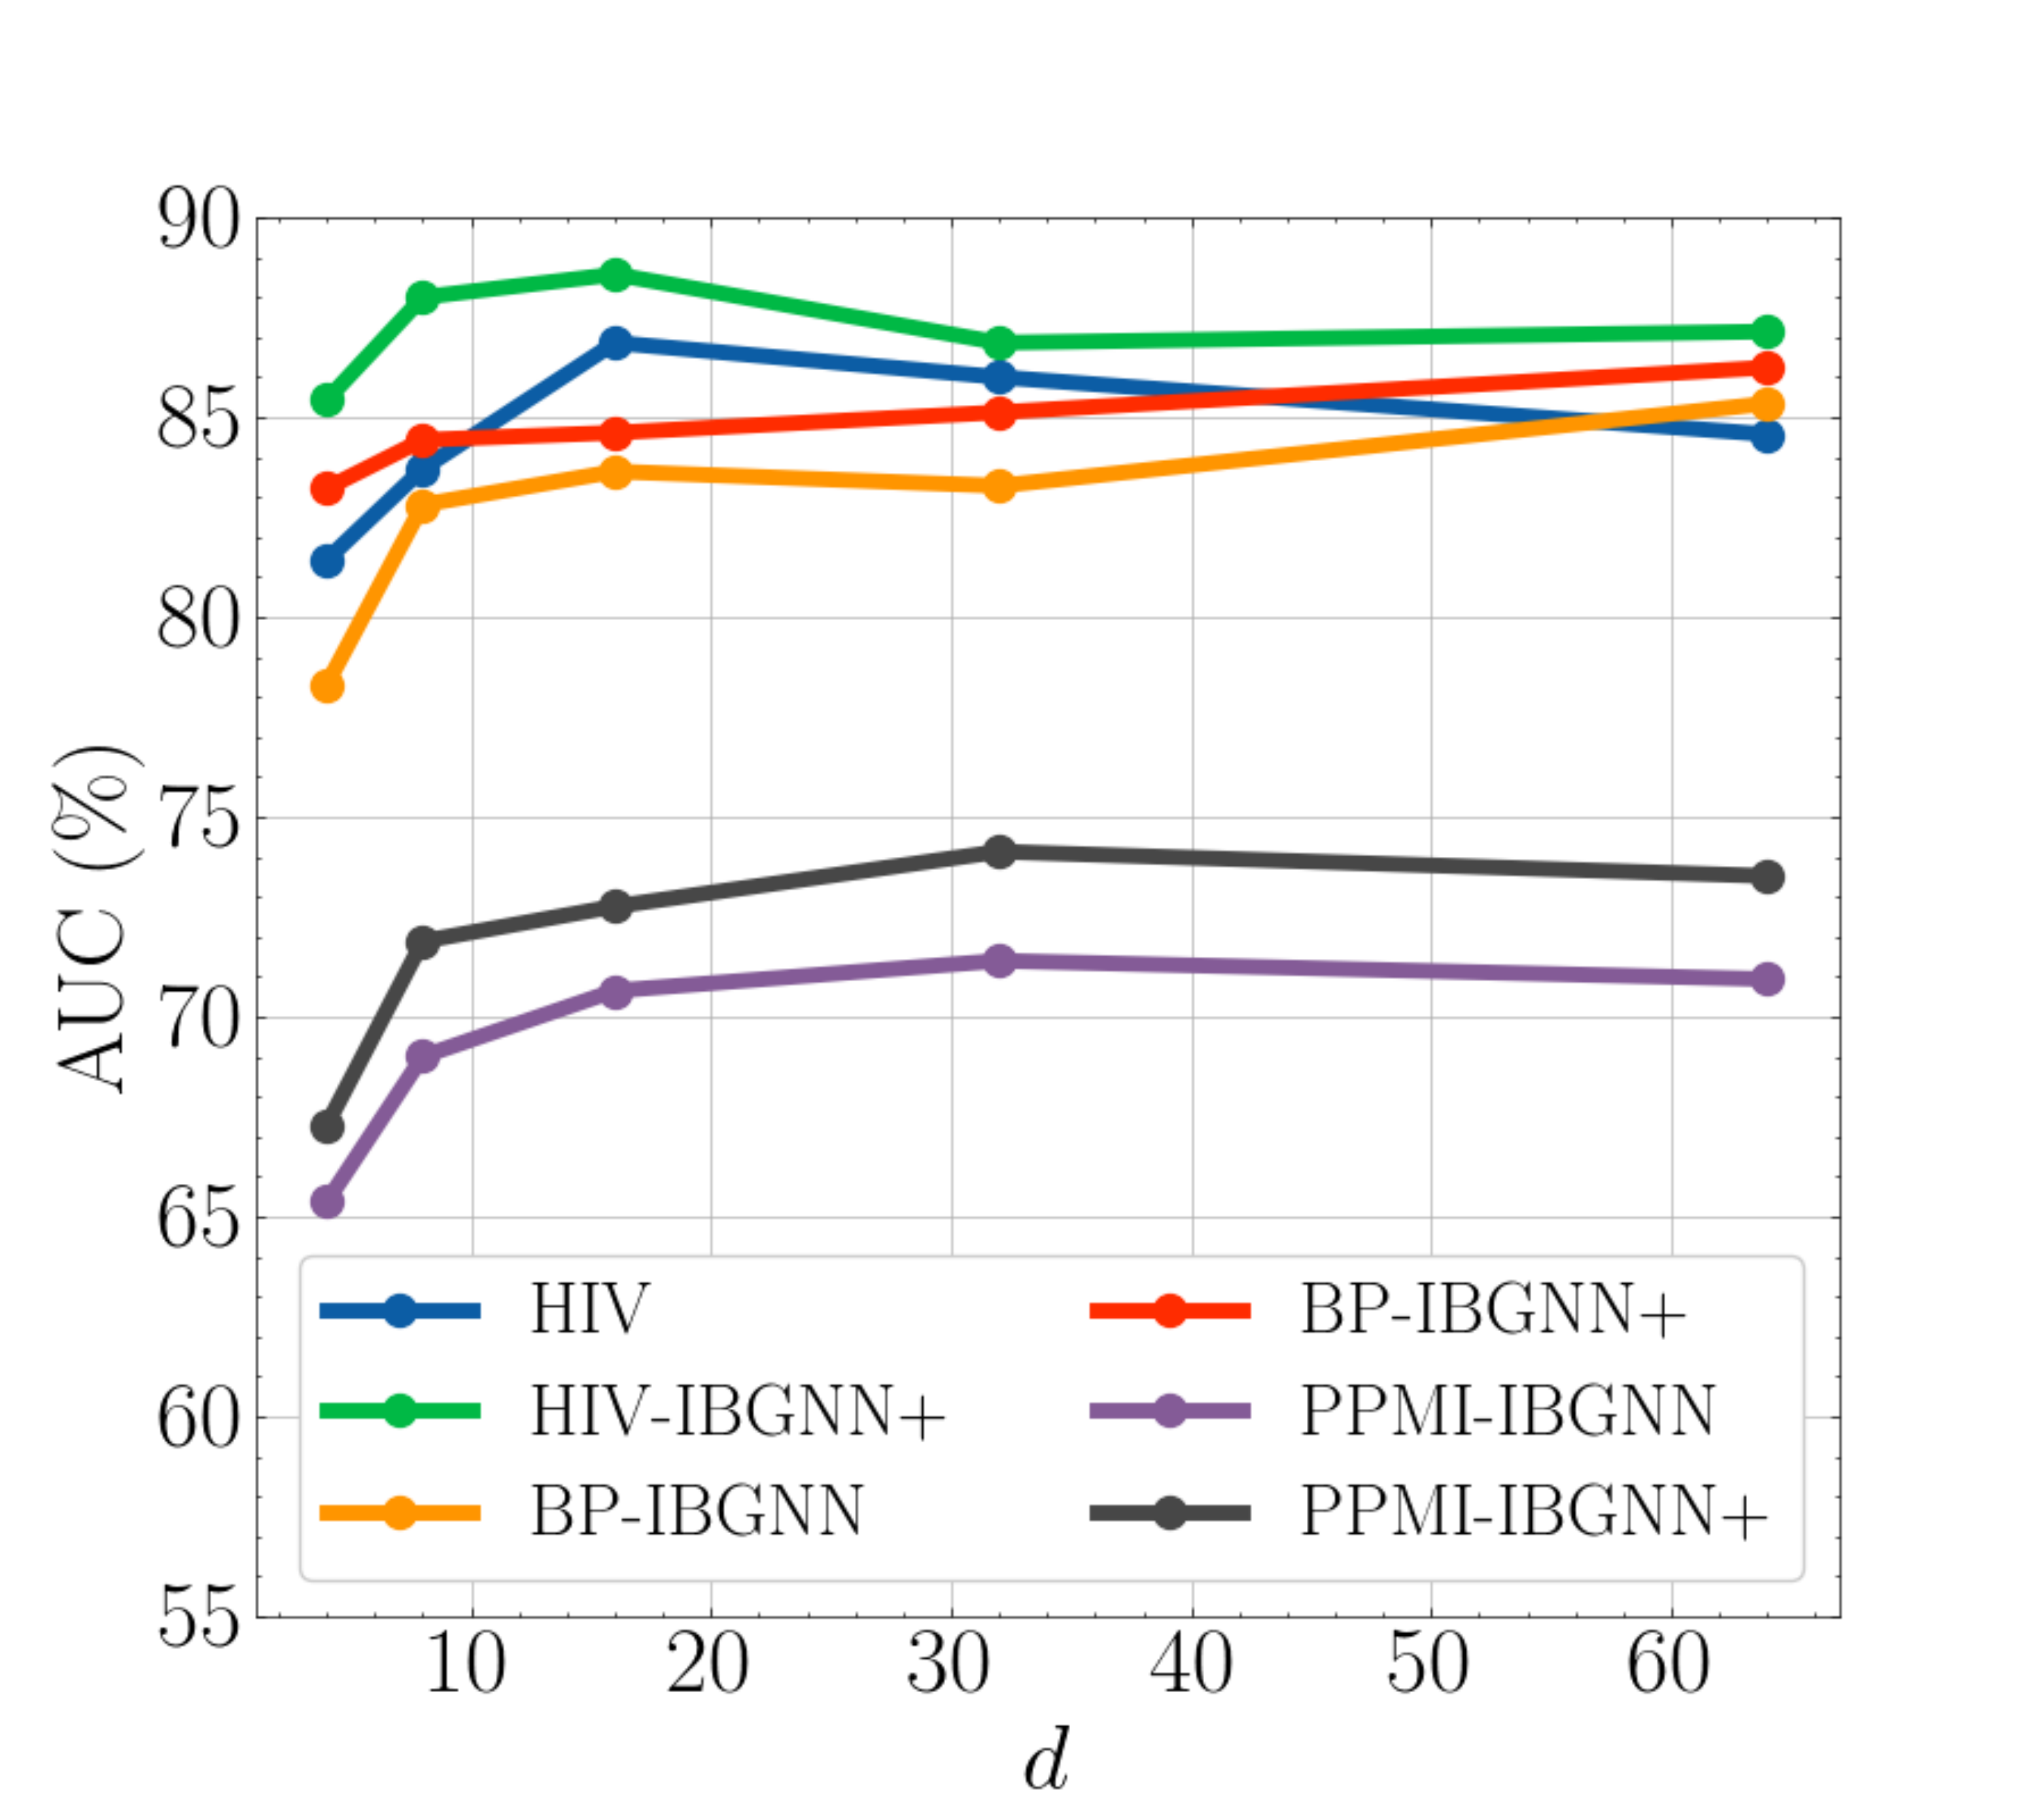}
      
      (b) Hidden dimension
      \label{fig:hiv_hc_nii}
    \end{minipage}%
\caption{\label{fig:sensitivity_vis} Sensitivity analysis of two main hyper-parameters. 
} 

\end{figure}

\section{Computation Cost}
\label{sec:supp-computational}
The average computational time ($s$) and memory footprint ($\text{MiB}$) of two standard deep baselines as well as our proposed models on three datasets are presented in Table \ref{tab:cost}. As shown in the table, our proposed backbone IBGNN takes the same amount of time and space as the basic GCN baseline and runs quicker than GAT on larger datasets PPMI, indicating that our proposed backbone prediction model is suitably efficient. The time complexity of the explanation enhanced model IBGNN\texttt{+} grows linearly compared with the backbone model by adding the explanation generator module and fine-tuning the backbone, and this feature is compatible with any backbone model beyond the one we presented.

\begin{table}[H]
	\centering
	\caption{The comparison of time and space computation cost between different methods on HIV, BP and PPMI datasets.}
	\resizebox{0.85\linewidth}{!}{
	\begin{tabular}{ccccccc}
	\toprule
	\multirow{2.5}{*}{Method} & \multicolumn{2}{c}{HIV} & \multicolumn{2}{c}{BP} & \multicolumn{2}{c}{PPMI} \\
	\cmidrule(lr){2-3} \cmidrule(lr){4-5} \cmidrule(lr){6-7}
		& Time ($s$) & Memory (MiB) & Time ($s$) & Memory (MiB) & Time ($s$) & Memory (MiB) \\
	\midrule
	GCN & 6.15 & 1113 & 5.68 & 1113 & 34.72 & 1113 \\
	GAT & 8.02 & 1119 & 8.60 & 1119 & 71.49 & 1093 \\
	IBGNN & 8.09 & 1121 & 8.10 & 1159 & 30.75 & 1113 \\
	IBGNN\texttt{+}  & 23.59 & 1147 & 22.76 & 1147 & 180.54 & 1117 \\
	\bottomrule
	\end{tabular}
	}
	\label{tab:cost}
\end{table}
